# Supplementary material for: SteP: Stacked LLM Policies for Web Actions
Source: arXiv:2310.03720 source file (2024-08-08)
Supplement: Supplementary file 1 [file autolabeling.tex]

\section{Autolabeling and Prompt Generation}
\label{sec:appendix:autolabeling}

We first collect a dataset of human demonstrations. We then ``autolabel'' each timestep with the low-level policy that was being executed. We convert the labelled datasets to prompts for both high-level planner and low-level policy. Finally, we augment prompts with chain-of-thought reasoning. 

% Given a dataset of raw demonstrations $\mathcal{D}=\{(\phi, s_1, a_1, \dots, s_T, a_T)\}$ of context, states and actions, the training objective is to generate prompts for both the task planner and a library of web policies. We do this by collecting and autolabeling demonstrations followed by autogenerating prompts from labeled demonstrations.

\subsection{Collect and Autolabel demonstrations}
We collect demonstrations from a human user who is given a conversation context $\phi$ and performs a sequence of actions in the browser to complete the task. We design a browser plugin to record webpage DOM $d$ and events such as clicks and types. Each demonstration is parsed as text by converting the DOM tree into a list of salient web elements like links, buttons, inputs. Each element is represented as text, e.g. \texttt{<button id=18 title="Travelers">1 Adult />}. Action events are parsed as a \texttt{CLICK <id>} or \texttt{TYPE <id> <val>}. The parsed demonstration dataset is represented as $\mathcal{D}=\{(\phi, s_1, a_1, \dots, s_T, a_T)\}$.

We then ``autolabel'' each timestep $t$ with a low-level policy $\pi_t$ and instruction $\psi_t$ to create a labeled dataset $(\phi, s_1, a_1, \color{black}\pi_1, \psi_1, \dots, s_T, a_T, \color{black}\pi_T, \psi_T)$. Ideally, to label full sequences, we would select the most likely sequence of policies given the entire state-action sequence $\arg \max_{\pi_{1:T}, \psi_{1:T}} \log P(\pi_1, \psi_1 \dots, \pi_T, \psi_T | s_1, a_1, \dots, s_T, a_T)$. However, this becomes impractical given demonstrations are too long to fit in to context length. Instead, we relax the problem to predicting the current policy given the previous policy, i.e. $\arg \max_{\pi_t} P(\pi_t | \pi_{t-1}, s_t, a_t)$.

% In the first stage, we convert unlabeled demonstrations $(\phi, s_1, a_1, \dots, s_T, a_T)$, into a labeled dataset by assigning a web policy $(\pi_t, \psi_t)$ at each time $t$ resulting in a labeled dataset $(\phi, s_1, a_1, \color{black}\pi_1, \psi_1\color{black}, \dots, s_T, a_T, \color{black}\pi_T, \psi_T\color{black})$. One way to do this is to have a human annotator assign a label, $(\pi_t, \psi_t)$, to every state--action $(s_t, a_t)$ pair. However, this process is tedious and time consuming for the annotator. Instead, we leverage LLMs to autolabel large sets of raw demonstrations using a few human annotations as examples.

% Ideally, to label full sequences, we would compute the probability of all policy labels $\pi_{1:T}$ given the entire state--action sequence, i.e. $P(\pi_1, \dots, \pi_T | s_1, a_1, \dots, s_T, a_T)$. However, this becomes impractical since demonstrations can be long with each state consisting of an entire web page DOM. Instead, we simplify the problem to predicting the current policy label given previous label and the next few state actions, i.e. $P(\pi_t | \pi_{t-1}, s_t, a_t, \dots, s_{t+k}, a_{t+k})$.

We construct an autolabeling prompt (Appendix~\ref{sec:appendix:autolabel_prompt}) that consists of an overall instruction along with a small set of human-annotated labels as in-context examples. Each in-context example has the following format: \texttt{\small \{input: [state $s_t$, action $a_t$, previous policy $\pi_{t-1})$], output: current policy $\pi_{t}$\}}.

%In-context example consists of the following:
% Context: Overall instruction describing the task, ɸ
% Current browser content: Browser content representing current state s_t
% Current action: Action a_t that the user demonstrated
% Previous label: Label assigned at previous time step. Since low-level policies can span multiple actions, having previous label is an informative feature for predicting current label
% Current label: Expected output from the LLM denoting low-level policy (\pi) and the instruction (\psi) for the policy. The format is \pi \psi, e.g. FILL_TEXT From " Boston ". For the in-context examples, the labels are manually annotated.

In-context examples are chosen such that they cover every low-level policy. We note that the auto-labeller can generalize to new tasks not contained in the prompt as long as the constituent low-level policies are covered (e.g. Search Flight $\rightarrow$ Cancel Booking) 

\subsection{Autogenerate prompts from labeled demonstrations}
Once we have a dataset of labeled demonstrations $\mathcal{D}_{label} = \{(\phi, s_0, a_0, (\pi_0, \psi_0), \dots, s_T, a_T, (\pi_T, \psi_T))\}$, we can use that to generate base prompts for both the high-level task planner and low-level policies. For the task planner, we concatenate the following input--output pairs as in-context examples in the base prompt: \texttt{\small \{input: [context $\phi$, initial state $s_0$]\}} and \texttt{\small \{output: sequence of web policy calls 
%$(\xi_1, \pi_1), (\xi_2, \pi_2) \dots, (\pi_T, \psi_T)$\}}. 
$(\pi_1, \psi_1), (\pi_2, \psi_2) \dots, (\pi_T, \psi_T)$\}}. 
For each web policy, we search the dataset $\mathcal{D}_{label}$ for all instances of the policy and create a prompt by concatenating examples of \texttt{\small \{input: [instruction $\psi_t$, current state $s_t$, previous actions $a_{t:t-k}$]\}} and \texttt{\small \{output: next action $a_t$\}}.

\subsection{Augmenting prompts with chain-of-thought reasoning}
Empirically, we observed that directly going from input browser content to output web actions can be difficult or error prone for the LLM. Chain-of-thought prompting \cite{wei2022chain} has shown to be effective to mitigate this. We additionally include a reasoning section between the input and output sections of the prompt that forces the LLM to generate a series of short sentences that provide justifications for the actions it predictions. We found this to uniformly improve performance for both task and policy prompts (Appendix~\ref{sec:appendix:ablations}). 
We subsequently added in a simple reason generator prompt (Appendix~\ref{sec:appendix:reasoning prompt}) that works across both high-level tasks and low-level policies. The prompt takes the current browser content $s_t$, previous actions $a_{t-1:t-k}$, current action $a_t$  and generates a reason $r$.

\subsection{Autolabeling Examples}

We include the following set of in-context examples for autolabeling that allows us to cover the different low-level policies:

\begin{enumerate}
    \item \textbf{MiniWoB:} In-context examples include 1 book flight demo, 1 search engine demo. This lets us cover \texttt{CHOOSE\_DATE()}, \texttt{FILL\_TEXT()}, \texttt{FIND\_AND\_CLICK\_SEARCH\_LINK()}, \texttt{FIND\_AND\_CLICK\_TAB\_LINK()} policies.
    \item \textbf{Airline CRM:} In-context examples include 1 demo of search flight, covering \texttt{CHOOSE\_DATE()}, \texttt{FILL\_TEXT()} policies.
    \item \textbf{LiveWeb:} In-context examples include 1 demo of book flight, covering \texttt{CHOOSE\_DATE()}, \texttt{FILL\_TEXT()}
\end{enumerate}
