# Supplementary material for: SteP: Stacked LLM Policies for Web Actions
Source: arXiv:2310.03720 source file (2024-08-08)
Supplement: Supplementary file 5 [file webarena.tex]

% \section{Webarena}
% \label{sec:appendix:webarena}
